# Supplementary material for: An Exploratory Analysis on the Explanatory Potential of Embedding-Based Measures of Semantic Transparency for Malay Word Recognition
Source: arXiv:2505.05973 ancillary file (2025-05-09)
Supplement: Supplementary file 1 [file Supplementary.pdf]

## Supplementary Materials

**Table S1**

*Model Concurvity (baseline)*

|          | Parametric | Word frequency*Root family size | Word length | Trial number, Subjects |
|----------|------------|---------------------------------|-------------|------------------------|
| Worst    | 1          | .81                             | .88         | 1.00                   |
| Observed | 1          | .46                             | .59         | .01                    |
| Estimate | 1          | .21                             | .50         | .00                    |

*Note.* Word frequency and root family size were log transformed. The model syntax is inverse RT ~ te(frequency\*family size) + s(word length) + experiment + s(trial number, subjects, bs= 'fs', m=1). Inverse RT = -1000/RT; a negative sign is used to make the interpretability more like traditional RT data.

**Table S2**

*Model Concurvity - LDA (Derived)*

|          | Parametric | Word frequency*Root family size | Word length | Trial number, Subjects |
|----------|------------|---------------------------------|-------------|------------------------|
| Worst    | 1          | .82                             | .89         | 1.00                   |
| Observed | 1          | .46                             | .59         | .01                    |
| Estimate | 1          | .21                             | .51         | .00                    |

*Note.* Word frequency and root family size were log transformed. The model syntax is inverse RT ~ te(frequency\*family size) + s(word length) + LDA-Derived+ experiment + s(trial number, subjects, bs= 'fs', m=1). Inverse RT = -1000/RT; a negative sign is used to make the interpretability more like traditional RT data

**Table S3**

*Model Concurvity - LDA (Shift)*

|          | Parametric | Word frequency*Root family size | Word length | Trial number, Subjects |
|----------|------------|---------------------------------|-------------|------------------------|
| Worst    | 1          | .82                             | .89         | 1.00                   |
| Observed | 1          | .46                             | .59         | .01                    |
| Estimate | 1          | .21                             | .51         | .00                    |

*Note.* Word frequency and root family size were log transformed. The model syntax is inverse RT ~ te(frequency\*family size) + s(word length) + LDA-Shift+ experiment + s(trial number, subjects, bs= 'fs', m=1). Inverse RT = -1000/RT; a negative sign is used to make the interpretability more like traditional RT data

**Table S4**

*Model Concurvity - Correlation (Derived Word and Centroid)*

|          | Parametric | Word frequency*Root family size | Word length | Correlation-dev.centroid | Trial number, Subjects |
|----------|------------|---------------------------------|-------------|--------------------------|------------------------|
| Worst    | 1          | .82                             | .90         | .33                      | 1.00                   |
| Observed | 1          | .52                             | .59         | .23                      | .01                    |
| Estimate | 1          | .24                             | .51         | .23                      | .00                    |

*Note.* Word frequency and root family size were log transformed. The model syntax is inverse RT ~ te(frequency\*family size) + s(word length) +s(correlation-dev.centroid) + experiment + s(trial number, subjects, bs= 'fs', m=1). Inverse RT = -1000/RT; a negative sign is used to make the interpretability more like traditional RT data

**Table S5**

*Model Concurvity - Correlation (Target Word and Predicted Word; FRACSS)*

|          | Parametric | Word frequency*Root family size | Word length | Correlation-FRACSS | Trial number, Subjects |
|----------|------------|---------------------------------|-------------|--------------------|------------------------|
| Worst    | 1          | .82                             | .89         | .46                | 1.00                   |
| Observed | 1          | .48                             | .59         | .20                | .01                    |
| Estimate | 1          | .22                             | .51         | .34                | .00                    |

*Note.* Word frequency and root family size were log transformed. The model syntax is inverse RT ~ te(frequency\*family size) + word length + s(correlation-FRACSS) + experiment + s(trial number, subjects, bs= 'fs', m=1). Inverse RT = -1000/RT; a negative sign is used to make the interpretability more like traditional RT data

**Table S6**

*Model Concurvity - Correlation (Derived Word and Shift)*

|          | Parametric | Word frequency*Root family size | Word length | Correlation-dev.shift | Trial number, Subjects |
|----------|------------|---------------------------------|-------------|-----------------------|------------------------|
| Worst    | 1          | .84                             | .89         | .38                   | 1.00                   |
| Observed | 1          | .57                             | .55         | .29                   | .01                    |
| Estimate | 1          | .26                             | .49         | .30                   | .00                    |

*Note.* Word frequency and root family size were log transformed. The model syntax is inverse RT ~ te(frequency\*family size) + word length + s(correlation- dev.shift) + experiment + s(trial number, subjects, bs= 'fs', m=1). Inverse RT = -1000/RT; a negative sign is used to make the interpretability more like traditional RT data

**Figure S1**

### t-SNE: Word Class (Adjective, Noun, Verb)

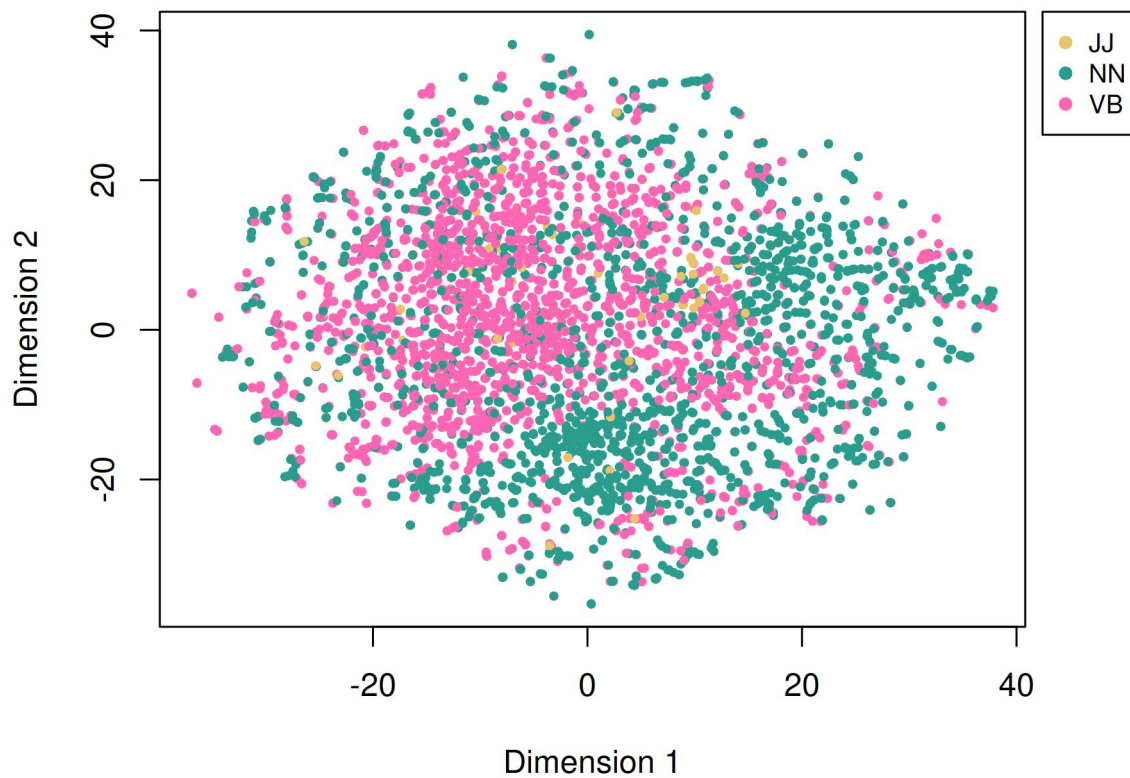

*Note.* Each coloured dot represents a derived word and each colour corresponds to a particular word category. JJ are adjectives ( $n = 763$ ), NN are nouns ( $n = 5065$ ), and VB are verbs ( $n = 2755$ ). Words that have similar embeddings appear closer to each other in the t-SNE space than others.
